# Supplementary material for: Molecular interpretation of the non-Newtonian viscoelastic behavior of liquid water at high frequencies
Source: arXiv:2003.08309 ancillary file (2020-03-18)
Supplement: Supplementary file 1 [file Supplemental_Material.pdf]

# Molecular interpretation of the non-Newtonian viscoelastic behavior of liquid water at high frequencies – Supplemental Material

Julius C. F. Schulz,[1] Alexander Schlaich,[1,2] Matthias Heyden,[3] Roland R. Netz,[1] and Julian Kappler[1,4,*]

[1] *Freie Universität Berlin, Fachbereich Physik, 14195 Berlin, Germany*
[2] *Université Grenoble Alpes, CNRS, LIPhy, 38000 Grenoble, France*
[3] *School of Molecular Sciences and Center for Biological Physics, Arizona State University, Tempe, Arizona 85287-1604, USA*
[4] *Department of Applied Mathematics and Theoretical Physics, University of Cambridge, Cambridge CB3 0WA, UK*

(Dated: March 18, 2020)

## CONTENTS

S1. Simulation Setup 1

S2. Calculating frequency-dependent viscosities 2
A. Linearized momentum conservation for an isotropic homogeneous continuum 2
B. Dynamics of the transverse velocity component 3
C. Viscosity in terms of the transversal velocity autocorrelation function 3
D. Approximate formula for small wave numbers 4
E. The Green-Kubo relation 4
F. Improving statistics for the Green-Kubo relation 5

S3. Fit of parallel combination of 3 Maxwell models + 1 shear inertia model to force field MD data 5

S4. Viscosity spectrum for SPC/E water 5

S5. Comparison of viscosity spectrum and orientational spectra 6

S6. Details for the calculation of the ab-initio MD water spectra 7

S7. Viscosity spectrum of a rigid-body Lennard-Jones fluid 8

References 8

## S1. SIMULATION SETUP

For the force field MD simulations in the main text, and unless noted otherwise also in this supplemental material, we use the GROMACS 4.6 molecular dynamics package[1], with an integration timestep 2 fs. Electrostatics are treated with PME[2]; a Verlet cutoff scheme is used, cutoff distance for potentials is 1 nm and dispersion corrections for energy and pressure are applied. Temperature is coupled to a v-rescale thermostat[3] at temperature $T = 300.2\,\mathrm{K}$. The system is preequilibrated at 1 atm in an NPT-ensemble simulation using a Parinello-Rahman barostat[4]. We simulate glycerol[5], modeled by the GROMOS53A6 force field[6], in TIP4P/2005 water[7]. Simulations are 250 ns long, and are performed in a 3 nm box using a NVT ensemble. For numerical evaluations of correlation functions and half-sided Fourier transforms we use a FFT algorithm.

* jkappler@physik.fu-berlin.de

## S2. CALCULATING FREQUENCY-DEPENDENT VISCOSITIES

In this section we derive relations for the shear viscosity in terms of velocity and stress tensor correlation functions. First, we use the linearized continuum-mechanical momentum conservation equation to obtain an equation for the dynamics of the transversal component of the fluid velocity field, i.e. the component perpendicular to the **k**-vector in Fourier space. Using this relation, we can express the shear viscosity in terms of the autocorrelation function of the transversal velocity field. In the small wave number limit, we derive an approximate simplified expression for the shear viscosity. Finally, we show that this latter expression reduces to the standard Green-Kubo relation[8–10] in the limit $\mathbf{k} \to 0$.

### A. Linearized momentum conservation for an isotropic homogeneous continuum

We start from the linearized continuum-mechanical momentum conservation equation[11],

$$\rho \dot{v}_\alpha(\mathbf{x}, t) = \sum_{\beta=1}^{3} \partial_\beta \sigma_{\alpha\beta}(\mathbf{x}, t), \qquad \alpha \in \{x, y, z\}, \tag{S1}$$

where $\rho$ is the constant equilibrium volume mass density of the fluid, $\mathbf{v}$ its velocity field, $\sigma$ its stress tensor, and a dot denotes a time derivative. Note that while for a compressible fluid the density is not constant, deviations from the equilibrium volume mass density $\rho$ on the left-hand side of Eq. (S1) would constitute nonlinear effects and are therefore not considered in our linear treatment. For a linear, homogeneous, isotropic compressible fluid the stress tensor is given as

$$\begin{aligned}\sigma_{\alpha\beta}(\mathbf{x}, t) = &-\delta_{\alpha\beta} P(\mathbf{x}, t) + 2 \int\int \eta(|\mathbf{x}'|, t') \dot{\epsilon}_{\alpha\beta}(\mathbf{x} - \mathbf{x}', t - t') \, \mathrm{d}^3\mathbf{x}' \, \mathrm{d}t' \\ &+ \delta_{\alpha\beta} \sum_{\gamma=1}^{3} \int\int \left( \eta'(|\mathbf{x}'|, t') - \frac{2}{3}\eta(|\mathbf{x}'|, t') \right) \dot{\epsilon}_{\gamma\gamma}(\mathbf{x} - \mathbf{x}', t - t') \, \mathrm{d}^3\mathbf{x}' \, \mathrm{d}t',\end{aligned} \tag{S2}$$

where $P$ is the pressure, the components of the rate of strain tensor $\dot{\epsilon}$ are

$$\dot{\epsilon}_{\alpha\beta} = \frac{1}{2}\left( \frac{\partial v_\alpha}{\partial x_\beta} + \frac{\partial v_\beta}{\partial x_\alpha} \right), \qquad \alpha, \beta \in \{x, y, z\}. \tag{S3}$$

and $\eta$, $\eta'$ are the shear and volume viscosity kernels, which for an isotropic medium only depend on the modulus of the vector $\mathbf{x}'$.

The model described by Eqs. (S1), (S2), is a generalization of the Newtonian fluid model, to which it reduces if the viscosity kernels decay fast as compared to the length- and time scales on which the strain tensor varies. In that case the strain tensors appearing in Eq. (S2) can be Taylor expanded around $(\mathbf{x}, t)$,

$$\begin{aligned}\dot{\epsilon}_{\alpha\beta}(\mathbf{x} - \mathbf{x}', t - t') \approx \dot{\epsilon}_{\alpha\beta}(\mathbf{x}, t) - \sum_{\gamma=1}^{3} x'_\gamma \frac{\partial \dot{\epsilon}_{\alpha\beta}}{\partial x_\gamma}(\mathbf{x}, t) \\ - t' \, \ddot{\epsilon}_{\alpha\beta}(\mathbf{x}, t).\end{aligned} \tag{S4}$$

Only keeping the lowest order term of this gradient expansion, Eq. (S2) reduces to

$$\begin{aligned}\sigma_{\alpha\beta}(\mathbf{x}, t) \approx &-\delta_{\alpha\beta} P(\mathbf{x}, t) + 2\bar{\eta}\dot{\epsilon}_{\alpha\beta}(\mathbf{x}, t) \\ &+ \delta_{\alpha\beta} \left( \bar{\eta}' - \frac{2}{3}\bar{\eta} \right) \sum_{\gamma=1}^{3} \dot{\epsilon}_{\gamma\gamma}(\mathbf{x}, t),\end{aligned} \tag{S5}$$

where

$$\bar{\eta} = \int\int \eta(|\mathbf{x}'|, t')\, \mathrm{d}^3\mathbf{x}'\, \mathrm{d}t', \tag{S6}$$

$$\bar{\eta}' = \int\int \eta'(|\mathbf{x}'|, t')\, \mathrm{d}^3\mathbf{x}'\, \mathrm{d}t', \tag{S7}$$

are the standard shear and volume viscosity which do not depend on space and time. A fluid whose stresses are given by Eq. (S5) is called a Newtonian fluid. If the stress tensor Eq. (S5) is used in the momentum conservation equation (S1), then the linearized compressible Navier-Stokes equation is recovered.

### B. Dynamics of the transverse velocity component

Inserting the stress-strain relation Eq. (S2) into the momentum conservation Eq. (S1) and applying a spatial Fourier transform, with convention

$$\hat{f}(\mathbf{k}) = \int f(\mathbf{x}) e^{i\mathbf{k}\cdot\mathbf{x}}\, \mathrm{d}^3\mathbf{x}, \quad \mathbf{k} \in \frac{2\pi}{L}\mathbb{Z}^3, \tag{S8}$$

$$f(\mathbf{x}) = \frac{1}{V}\sum_{\mathbf{k}} \hat{f}(\mathbf{k}) e^{-i\mathbf{k}\cdot\mathbf{x}}, \tag{S9}$$

where $V = L^3$ is the volume of the periodic simulation cube and $L$ the length of its sides, we obtain

$$\rho\partial_t \hat{v}_\alpha = (-ik_\alpha)\left[-\hat{P} + \left(\hat{\eta}' - \frac{2}{3}\hat{\eta}\right) \circledast \left(\sum_{\gamma=1}^{3} \hat{\epsilon}_{\gamma\gamma}\right)\right] + \sum_{\beta=1}^{3}(-ik_\beta) 2\hat{\eta} \circledast \hat{\epsilon}_{\alpha\beta}, \tag{S10}$$

where the symbol $\circledast$ denotes a temporal convolution and we denote spatial Fourier transforms by a hat. As before we assume the medium to be isotropic, so that the viscosities only depend on the modulus of $\mathbf{k}$, i.e. $\hat{\eta}(\mathbf{k}, t) \equiv \hat{\eta}(k, t)$, $\hat{\eta}'(\mathbf{k}, t) \equiv \hat{\eta}'(k, t)$, where $k := |\mathbf{k}|$.

Defining longitudinal and transversal projection operators

$$\mathcal{P}^{\parallel}_{\alpha\beta} = \frac{k_\alpha k_\beta}{k^2}, \tag{S11}$$

$$\mathcal{P}^{\perp}_{\alpha\beta} = \delta_{\alpha\beta} - \mathcal{P}^{\parallel}_{\alpha\beta}, \tag{S12}$$

and applying $\mathcal{P}^{\perp}$ to Eq. (S10), we obtain

$$\rho\partial_t \hat{v}^{\perp}_\alpha = -k^2 \hat{\eta} \circledast \hat{v}^{\perp}_\alpha, \tag{S13}$$

where $\hat{v}^{\perp}_\alpha := \sum_\beta \mathcal{P}^{\perp}_{\alpha\beta}\hat{v}_\beta$ and we use that

$$\sum_{\beta=1}^{3} \mathcal{P}^{\perp}_{\alpha\beta}\hat{\epsilon}_{\beta\gamma} = \frac{1}{2}\sum_{\beta=1}^{3} \mathcal{P}^{\perp}_{\alpha\beta}\left[(-ik_\beta)\hat{v}_\gamma + (-ik_\gamma)\hat{v}_\beta\right] \tag{S14}$$

$$= \frac{1}{2}(-ik_\gamma)\sum_{\beta=1}^{3} \mathcal{P}^{\perp}_{\alpha\beta}\hat{v}_\beta \tag{S15}$$

$$= \frac{1}{2}(-ik_\gamma)\hat{v}^{\perp}_\alpha. \tag{S16}$$

Applying a half-sided temporal Fourier transform, defined by

$$\tilde{f}(\mathbf{k}, \omega) = \int_0^\infty e^{-i\omega t} \hat{f}(\mathbf{k}, t)\, \mathrm{d}t, \tag{S17}$$

to Eq. (S13), we obtain

$$i\omega\rho\tilde{v}^{\perp}_\alpha - \rho\hat{v}^{\perp}_\alpha(0) = -k^2\tilde{\eta}\tilde{v}^{\perp}_\alpha, \tag{S18}$$

where we denote the combined spatial Fourier and temporal half-sided Fourier transform by a tilde. Equation (S18) can readily be solved for $\tilde{v}^{\perp}_\alpha$ to yield

$$\tilde{v}^{\perp}_\alpha(\mathbf{k}, \omega) = \frac{\hat{v}^{\perp}_\alpha(\mathbf{k}, 0)}{i\omega + k^2\tilde{\eta}(\mathbf{k}, \omega)/\rho}. \tag{S19}$$

This is an equation for the dynamics of the transversal velocity field, i.e. the shearing part of the velocity field.

### C. Viscosity in terms of the transversal velocity autocorrelation function

We define the normalized autocorrelation function of the $\alpha$-component of the transversal velocity,

$$\hat{C}^{\perp}(\mathbf{k}, t) = \frac{\langle \hat{v}^{\perp}_\alpha(\mathbf{k}, t)\ \hat{v}^{\perp}_\alpha(-\mathbf{k}, 0)\rangle}{\langle \hat{v}^{\perp}_\alpha(\mathbf{k}, 0)\ \hat{v}^{\perp}_\alpha(-\mathbf{k}, 0)\rangle}, \tag{S20}$$

whose half-sided Fourier transform, using Eq. (S19), becomes

$$\tilde{C}^{\perp}(\mathbf{k}, \omega) = \frac{1}{i\omega + k^2\tilde{\eta}(k, \omega)/\rho}. \tag{S21}$$

Note that this equation does not depend on the component $\alpha$ anymore, which is why we have omitted a subscript $\alpha$ for $\hat{C}^{\perp}$. Also note that this equation shows that for an isotropic material, $\tilde{C}$ actually only depends on the modulus of $\mathbf{k}$, $\tilde{C}(\mathbf{k}, \omega) \equiv \tilde{C}(k, \omega)$.

Solving for $\tilde{\eta}$, we obtain[9]

$$\tilde{\eta}(k, \omega) = -\frac{i\omega\rho}{k^2}\left(1 - \frac{1}{i\omega\,\tilde{C}^{\perp}(k, \omega)}\right). \tag{S22}$$

This is an exact expression for the shear viscosity in terms of the autocorrelation function $\tilde{C}^{\perp}$.

### D. Approximate formula for small wave numbers

For small wave numbers, an approximation to Eq. (S22) can be derived. Assuming

$$\left|\frac{k^2\tilde{\eta}}{\rho\omega}\right| \ll 1, \tag{S23}$$

and using $1/(1+x) \approx 1-x$ ($|x| \ll 1$), Eq. (S21) can be approximated as

$$\tilde{C}^{\perp} \approx \frac{1}{i\omega}\left(1 - \frac{k^2\tilde{\eta}}{i\omega\rho}\right) = \tag{S24}$$

$$= \frac{1}{i\omega} + \frac{k^2\tilde{\eta}}{\rho\omega^2}, \tag{S25}$$

which, after solving for $\tilde{\eta}$, yields

$$\tilde{\eta}(k,\omega) = \frac{\rho}{k^2}\left(i\omega + \omega^2\tilde{C}^{\perp}(k,\omega)\right). \tag{S26}$$

We can further simplify the right-hand side of this equation. For this, we use the relation

$$\widetilde{\partial_t^2 f}(\omega) = -\omega^2\tilde{f}(\omega) - i\omega f(t=0) - (\partial_t f)(t=0) \tag{S27}$$

between the half-sided Fourier transform of the second derivative of a function and the half-sided Fourier transform of the function itself, to rewrite

$$i\omega + \omega^2\tilde{C}^{\perp}(k,\omega) = (\partial_t\hat{C}^{\perp})(k,0) + i\omega\hat{C}^{\perp}(k,0) + \omega^2\tilde{C}^{\perp}(k,\omega) \tag{S28}$$

$$= -\widetilde{\partial_t^2\hat{C}^{\perp}}(k,\omega). \tag{S29}$$

where we use $\hat{C}^{\perp}(k,0) = 1$, c.f. Eq. (S20), and $\partial_t\hat{C}^{\perp}(k,0) = 0$, since $\hat{C}$ is an even and analytic function of $t$. Substituting Eq. (S29) into the right-hand side of Eq. (S26) and writing out the half-sided Fourier transform explicitly, we obtain[9]

$$\tilde{\eta}(k,\omega) = -\frac{\rho}{k^2}\int_0^\infty e^{-i\omega t}\ (\partial_t^2\hat{C}^{\perp})(k,t)\ \mathrm{d}t. \tag{S30}$$

As mentioned before, this formula is only valid in the small wave number limit. As a numerical example, if we assume bulk water values, $|\tilde{\eta}| \approx 0.1\ \mathrm{mPa\cdot s}$, $\rho = 10^3\ \mathrm{kg/m^3}$, then condition (S23) becomes

$$|k|^2\frac{\mathrm{nm}^2}{\mathrm{ps}} \ll |\omega|. \tag{S31}$$

Thus, for $|k| = 4\ \mathrm{nm}^{-1}$, corresponding to the smallest wave number resolvable in a typical box in an MD simulation, the relation Eq. (S30) is valid for

$$\omega \gg 1.6\ \frac{1}{\mathrm{ps}}, \tag{S32}$$

i.e. for frequencies well above 1 THz, which severly limits the applicability of Eq. (S30).

Note however that in the limit $\mathbf{k} \to 0$, condition Eq. (S23) is always fulfilled, and the approximate Eq. (S30) is valid. However, obtaining $\hat{v}_\alpha^{\perp}$ in this limit from MD simulations is typically difficult because a large simulation box is required.

### E. The Green-Kubo relation

We now show that in the limit $\mathbf{k} \to 0$, Eq. (S30) reduces to the standard Green-Kubo relation for the shear viscosity. In order to do this, we use momentum conservation to replace the second derivative of the transversal velocity autocorrelation function $\hat{C}^{\perp}(\mathbf{k},t)$ in Eq. (S30) by a stress-tensor autocorrelation function.

First, we note that[12]

$$\partial_t^2\langle\hat{v}_\alpha^{\perp}(\mathbf{k},t)\ \hat{v}_\alpha^{\perp}(-\mathbf{k},0)\rangle = -\langle\dot{\hat{v}}_\alpha^{\perp}(\mathbf{k},t)\ \dot{\hat{v}}_\alpha^{\perp}(-\mathbf{k},0)\rangle, \tag{S33}$$

where $\alpha \in \{x,y,z\}$. Furthermore, Eq. (S13) yields, for any $\alpha \neq \beta$ and wave vector $\mathbf{k} = k\mathbf{e}_\beta$, that

$$\dot{\hat{v}}_\alpha^{\perp}(\pm\mathbf{k},t) = \mp\frac{ik}{\rho}\hat{\sigma}_{\alpha\beta}(\pm\mathbf{k},t), \tag{S34}$$

where we use

$$\sum_{\lambda,\gamma=1}^{3} k_\lambda\mathcal{P}_{\alpha\gamma}^{\perp}\hat{\sigma}_{\gamma\lambda} = k\sum_{\gamma=1}^{3}\mathcal{P}_{\alpha\gamma}^{\perp}\hat{\sigma}_{\gamma\beta} \tag{S35}$$

$$= k\sum_{\gamma=1}^{3}\delta_{\alpha\gamma}\hat{\sigma}_{\gamma\beta} = k\hat{\sigma}_{\alpha\beta}. \tag{S36}$$

Using Eq. (S34) to eliminiate $\dot{\hat{v}}_\alpha^{\perp}$ in Eq. (S33), and substituting the result into the correlation function in Eq. (S30), we obtain

$$\tilde{\eta}(\mathbf{k} = k\mathbf{e}_\beta,\omega) = \frac{1}{\langle\hat{v}_\alpha(\mathbf{k},0)\hat{v}_\alpha(-\mathbf{k},0)\rangle\rho}\times \int_0^\infty e^{-i\omega t}\ \langle\hat{\sigma}_{\alpha\beta}(\mathbf{k},t)\hat{\sigma}_{\alpha\beta}(-\mathbf{k},0)\rangle\ \mathrm{d}t, \tag{S37}$$

where we use that, according to Eq. (S12), for $\alpha \neq \beta$ it holds that $\hat{v}_\alpha^{\perp}(\mathbf{k},0) = \hat{v}_\alpha(\mathbf{k},0)$.

In the limit $\mathbf{k} \to 0$, we can further rewrite this expression. First, for any two observables $f$, $g$ (functions defined in the simulation box), it holds that[13]

$$\lim_{\mathbf{k}\to\mathbf{0}}\langle\hat{f}(\mathbf{k},0)\hat{g}(-\mathbf{k},0)\rangle = V^2\langle fg\rangle, \tag{S38}$$

where the average on the right-hand side is not only over the ensemble, but also an averaged correlation of $f$, $g$ over all of space, i.e.

$$\langle fg\rangle \equiv \frac{1}{V^2}\int \mathrm{d}^3\mathbf{x}\int \mathrm{d}^3\mathbf{y}\ \langle f(\mathbf{x})g(\mathbf{y})\rangle_{\text{ensemble}}, \tag{S39}$$

where we have explicitly marked the ensemble average here. This identity allows to replace the Fourier transformed velocity and stress tensor correlations by real-space averages in the limit of vanishing wave vector.

Second, for the center of mass velocity of the whole fluid, the equipartition theorem yields

$$\rho V \langle v_\alpha^2 \rangle = k_\mathrm{B} T, \quad \alpha \in \{x, y, z\}, \tag{S40}$$

so that, combining Eqs. (S39), (S40), we get

$$\lim_{\mathbf{k}\to\mathbf{0}} \langle \hat{v}_\alpha(\mathbf{k}, 0)\hat{v}_\alpha(-\mathbf{k}, 0)\rangle = k_\mathrm{B} T \frac{V}{\rho}. \tag{S41}$$

Thus, in the limit $\mathbf{k} \to \mathbf{0}$, Eq. (S37) can be rewritten as

$$\tilde{\eta}(\mathbf{k} = 0, \omega) = \frac{V}{k_\mathrm{B} T} \int_0^\infty e^{-i\omega t} \left\langle \sigma_{\alpha\beta}(t)\sigma_{\alpha\beta}(0) \right\rangle \mathrm{d}t, \tag{S42}$$

where the average on the right hand side is to be understood as an averaged correlation function over all of space, c.f. Eq. (S39), and we stress that $\alpha \neq \beta$. This is the well known Green-Kubo relation[8–10].

Since the above formula holds for any off-diagonal element of the stress tensor, one can improve statistics in a numerical evaluation of Eq. (S43) by calculating an average over all 6 possible combinations for $\alpha \neq \beta$, i.e.

$$\tilde{\eta}(\mathbf{k} = 0, \omega) = \frac{V}{6 k_\mathrm{B} T} \int_0^\infty e^{-i\omega t} \sum_{\alpha\neq\beta} \left\langle \sigma_{\alpha\beta}(t)\sigma_{\alpha\beta}(0) \right\rangle \mathrm{d}t. \tag{S43}$$

### F. Improving statistics for the Green-Kubo relation

Analogously to the calculations leading to Eq. (S43), projecting the momentum conservation equation (S10) onto the longitudinal part using $\mathcal{P}^{||}_{\alpha\beta}$, c.f. Eq. (S11), and considering longitudinal velocity autocorrelation functions in the limit $\mathbf{k} \to 0$, it can be shown[9] that each diagonal element of the trace free part of the stress tensor,

$$\Pi_{\alpha\beta} = \sigma_{\alpha\beta} - \delta_{\alpha\beta} \frac{1}{3} \sum_\gamma \sigma_{\gamma\gamma} \quad \alpha, \beta \in \{x, y, z\}, \tag{S44}$$

can also be used to calculate the viscosity according to

$$\frac{4}{3}\tilde{\eta}(\mathbf{k} = 0, \omega) = \frac{V}{k_\mathrm{B} T} \int_0^\infty e^{-i\,\omega\,t} \left\langle \Pi_{\alpha\alpha}(t)\,\Pi_{\alpha\alpha}(0) \right\rangle \mathrm{d}t, \tag{S45}$$

$\alpha \in \{x, y, z\}$. Combining Eqs. (S43), (S45), one thus arrives at the formula[9,14–16]

$$\tilde{\eta}(\mathbf{k} = 0, \omega) = \frac{V}{10\, k_\mathrm{B} T} \times \int_0^\infty e^{-i\,\omega\,t} \sum_{\alpha\beta} \left\langle \Pi_{\alpha\beta}(t)\,\Pi_{\alpha\beta}(0) \right\rangle \mathrm{d}t, \tag{S46}$$

which uses all components of the stress tensor and therefore improves statistics even further as compared to Eq. (S43). For numerical evaluation of the viscosity we use Eq. (S46), correlation functions and half-sided Fourier transforms are calculated using a FFT algorithm.

Note that in the limit $\omega \to 0$, Eq. (S46) becomes[8–10,14–16]

$$\bar{\eta} = \frac{V}{10\, k_B\, T} \int_0^\infty \sum_{\alpha\beta} \left\langle \Pi_{\alpha\beta}(t)\,\Pi_{\alpha\beta}(0) \right\rangle \mathrm{d}t. \tag{S47}$$

## S3. FIT OF PARALLEL COMBINATION OF 3 MAXWELL MODELS + 1 SHEAR INERTIA MODEL TO FORCE FIELD MD DATA

In the present section we consider a viscoelastic network comprised of a parallel combination of three Maxwell models and one shear inertia model. The total viscosity of this network is given by

$$\tilde{\eta}(\omega) = \sum_{j=\mathrm{I,II,IV}} \frac{\eta_{0,j}}{1 - i\omega\tau_j} + \eta_{0,\mathrm{III}} \frac{1 - i\omega\tau_{m,\mathrm{III}}}{1 - i\omega\tau_{0,\mathrm{III}}^2/\tau_{m,\mathrm{III}} - \omega^2\tau_{0,\mathrm{III}}^2}. \tag{S48}$$

The result of a fit of this model to the force field MD data is shown in Fig. S1 (a), the resulting parameters are given in Table I. As Fig. S1 (a) shows, this viscoelastic network is able to reproduce the MD spectrum quite well. This is in agreement with the discussion in the main text, where a parallel combination of two Maxwell models and two shear inertia models is used; there, it is found that one of the shear inertia models is in fact overdamped.

## S4. VISCOSITY SPECTRUM FOR SPC/E WATER

In this section, we discuss the robustness of our results with regards to the underlying water model. In Fig. S2 we compare viscosity spectra obtained from TIP4P/2005 and SPC/E[17] water models.

As the figure shows, the spectra are qualitatively very similar; in particular they both produce the high frequency peak in the real- and imaginary parts

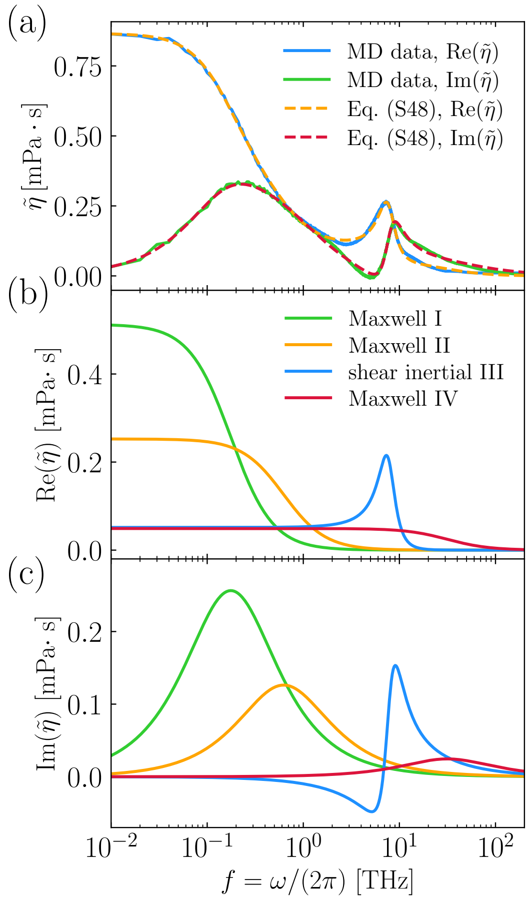


FIG. S1. **(a):** Complex viscosity $\tilde{\eta}$ from MD simulations compared to the fitted viscoelastic network. The viscoelastic network is a parallel combination of an shear inertia model and three Maxwell models. The resulting complex viscosity is given by Eq. (S48), the fitting parameters are given in Table I. **(b), (c):** Real and imaginary part of the individual constituents (one shear inertia model, three Maxwell models) that are connected in parallel to yield the viscosity shown in subplot (a).

TABLE I. Fitting parameters for the viscoelastic model Eq. (S48), fit to TIP4P/2005 water, c.f. Fig. S1. Timescales are converted to frequencies via $f = (2\pi\tau)^{-1}$ for ease of comparison with Fig. S1.

| Parameter | Value |
|---|---|
| $\eta_{0,\mathrm{I}}$ | 0.513 mPa · s |
| $(2\pi \cdot \tau_{\mathrm{I}})^{-1}$ | 0.18 THz |
| $\eta_{0,\mathrm{II}}$ | 0.252 mPa · s |
| $(2\pi \cdot \tau_{\mathrm{II}})^{-1}$ | 0.62 THz |
| $\eta_{0,\mathrm{III}}$ | 0.052 mPa · s |
| $(2\pi \cdot \tau_{m,\mathrm{III}})^{-1}$ | 3.96 THz |
| $(2\pi \cdot \tau_{0,\mathrm{III}})^{-1}$ | 7.83 THz |
| $\eta_{0,\mathrm{IV}}$ | 0.049 mPa · s |
| $(2\pi \cdot \tau_{\mathrm{IV}})^{-1}$ | 31.53 THz |

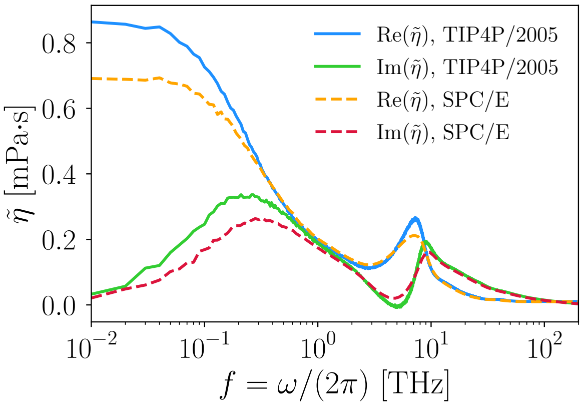


FIG. S2. Viscosity spectra obtained from TIP4P/2005 (solid colored lines; replot of Fig. 4 (a) of the main text) and SPC/E (dashed colored lines) water models, c.f. Sect. S4. For both systems, the viscosity is calculated from the MD data using Eq. (S46). For the dashed lines, a cubic box of edge length 4 nm filled with SPC/E water is simulated in an NVT ensemble for 250 ns. As in the TIP4P/2005 simulations, for the SPC/E simulations the temperature is set to $T = 300.2\,\mathrm{K}$ via a v-rescale thermostat[3].

of the viscosity around 10 THz. The spectral features we investigate in the present work are thus present in both water models considered.

More quantitatively, the amplitude and thus the steady-state shear viscosity is smaller in the SPC/E water model. Also the frequency of the Maxwell peak ($f \approx 0.2$ THz) is slightly lower in the SPC/E water model, wheras the position of the high frequency peak ($f \approx 10$ THz) is unaltered. While the position of this peak is independent of the water model, the detailed shape of this high-frequency peak does depend on the water model used.

## S5. COMPARISON OF VISCOSITY SPECTRUM AND ORIENTATIONAL SPECTRA

In the main text we associate the shoulder at $f \approx 20$ THz in the viscosity spectrum with rotational vibrations of individual water molecules within the force field of their surrounding molecules. To infer the typical timescale of rotations of individual water molecules, we calculate the corresponding orientational spectra. We define the normalized dipole

vector of atom $i$,

$$\mathbf{P}^i_{HOH} = \frac{(\mathbf{H}^i_1 + \mathbf{H}^i_2)/2 - \mathbf{O}^i}{\left|(\mathbf{H}^i_1 + \mathbf{H}^i_2)/2 - \mathbf{O}^i\right|}, \tag{S49}$$

where $\mathbf{H}^i_1, \mathbf{H}^i_2, \mathbf{O}^i$ are the positions of the three atoms of the $i$-th water molecule. Additionally, we define the two orthogonal vectors

$$\mathbf{P}^i_{HH} = \frac{\mathbf{H}^i_1 - \mathbf{H}^i_2}{\left|\mathbf{H}^i_1 - \mathbf{H}^i_2\right|} \tag{S50}$$

$$\mathbf{P}^i_{\perp} = \mathbf{P}^i_{HOH} \times \mathbf{P}^i_{HH}, \tag{S51}$$

where $\times$ denotes the standard cross product on $\mathbb{R}^3$, so that $\mathbf{P}^i_{HOH}$, $\mathbf{P}^i_{HH}$, $\mathbf{P}^i_{\perp}$ is an oriented orthonormal frame fixed to water molecule $i$. We then calculate the correlation functions

$$\phi_{HOH}(t) = \sum_i \left\langle \mathbf{P}^i_{HOH}(t) \cdot \mathbf{P}^i_{HOH}(0) \right\rangle, \tag{S52}$$

$$\phi_{HH}(t) = \sum_i \left\langle \mathbf{P}^i_{HH}(t) \cdot \mathbf{P}^i_{HH}(0) \right\rangle, \tag{S53}$$

$$\phi_{\perp}(t) = \sum_i \left\langle \mathbf{P}^i_{\perp}(t) \cdot \mathbf{P}^i_{\perp}(0) \right\rangle, \tag{S54}$$

where the sum is over all water molecules in the system and the dot denotes the scalar product. The imaginary part of the half-sided Fourier transformed correlation functions together with $\mathrm{Im}(\tilde{\eta})$ are shown in Fig. S3. The orientational spectra show two peaks, one at around $10^{-2}$ THz, corresponding to slow reorientation of water molecules, corresponding to the microwave Debye peak, and one at around 20 THz, corresponding to orientational vibrations. The latter peak occurs at a similar frequency as the Maxwell model IV peak, so that we conclude that the microscopic origin of this feature of the viscosity spectrum are librational excitations of water molecules.

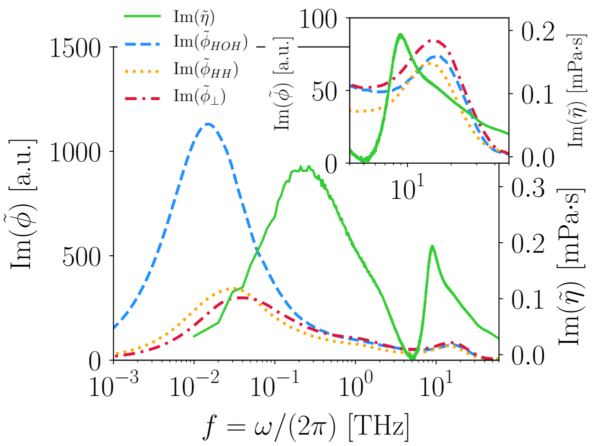


FIG. S3. **Comparison of viscosity and orientational spectra.** The main figure shows the imaginary part of the half-sided Fourier transforms of the correlation functions $\phi_{HOH}$, $\phi_{HH}$, $\phi_{\perp}$, which are defined by Eqs. (S52), (S53), (S54), together with the imaginary part of the viscosity spectrum, a replot of the green curve shown in Fig. 4 (a) of the main text. The inset shows a zoom-in on the frequencies around 20 THz with the relative scales of viscosity and orientational spectra adapted to show that the frequency of the high frequency peaks in the orientational spectra coincides with the feature in the complex viscosity modeled by Maxwell model IV, c.f. Fig. 4 (e) of the main text.

## S6. DETAILS FOR THE CALCULATION OF THE AB-INITIO MD WATER SPECTRA

In the present section we give details for the ab-initio QM/MM simulations[18,19] (aiMD) used to calculate the viscosity spectrum. We furthermore compare spectra calculated from force field MD simulations, with system size comparable to the aiMD system and using the same analysis protocol as used for the aiMD data, to the viscosity spectrum discussed in the main text.

The aiMD system is comprised of 128 water molecules in a box with edge length $L = 1.56\,\mathrm{nm}$, corresponding to a smallest wave number $k = 2\pi/L = 4.016\,\mathrm{nm}^{-1}$; in total, 16 trajectories with 20 ps length each are simulated[18]. As no pairwise forces are available, the virial for the periodic system aiMD cannot be calculated, and thus the spectrum cannot be evaluated at $k = 0$ using Eq. (S46).

However, the spectrum at finite $k$ can be computed. From the aiMD trajectories, the transversal current can be calculated via

$$\hat{\mathbf{j}}^{\perp}(\mathbf{k}, t) = \sum_i m_i \, \mathbf{v}_i^{\perp} \, e^{i\,\mathbf{k}\cdot\mathbf{r}_i(t)}, \tag{S55}$$

with

$$\mathbf{v}_i^{\perp} = \mathbf{v}_i - \mathbf{k}\frac{\mathbf{k}\cdot\mathbf{v}_i}{\mathbf{k}^2}, \tag{S56}$$

where $\mathbf{v}_i$, $m_i$, $\mathbf{r}_i$ are the velocity, mass, and position of the $i$-th nucleus, and the sum in Eq. (S55) extends over all nuceli in the system. The normalized autocorrelation function of the transversal current can then be used in Eq. (S22), or the approximate Eq. (S30), to obtain $\tilde{\eta}(k, \omega)$ at finite wave number $k$.

To validate this method, we also consider a force field MD system similar to the aiMD setup. The force field MD system is comprised of 128 TIP4P/2005 water molecules in a cubic box with edge length $L = 1.56$ nm, and an interaction cutoff distance 0.75 nm. The resulting viscosity spectra

of both MD and aiMD data are shown in Fig. S4. For comparison, all subplots also feature the $k = 0$ spectrum shown in Fig. 4 (a) of the main text.

In the upper row of Fig. S4 we compare spectra from MD simulations in a small box at finite $k = 4.016$ nm$^{-1}$ to the $k = 0$ results obtained via Eq. (S46) in the larger box considered in the main text. In Fig. S4 (a) we see that even for a small finite $k$-value, the spectrum remains almost unaltered, except for a small $k$-dependence of the steady-state shear viscosity (low-frequency limit of real part in subplot (a)); this deviation should scale as $k^2$, as argued by Palmer[20]. In Fig. S4 (b) we see that also the spectrum calculated using Eq. (S30) for finite $k$ agrees very well with its $k = 0$ counterpart. Note that, as discussed in Sect. S2 D, the approximate formula Eq. (S30) is only applicable for $f \gg 1$ THz, which explains the breakdown of the finite-$k$ results at $f \approx 0.3$ THz.

In the lower row of Fig. S4, the MD spectrum at $k = 0$ is compared to the finite-$k$ spectrum obtained from aiMD. Due to the limited statistics, the low-frequency regime is not well described. However, one can see that in both subplots (c) and (d), the feature at $f \approx 10$ THz is present in the ab-initio simulations, and appears at a similar frequency as in the force field MD water models. Note, however, that the imaginary part has a different shape, and that the amplitude of the spectrum in the ab-initio simulation is larger (note in this context that the TIP4P/2005 steady state shear viscosity is lower than the experimental value). The aiMD spectrum also shows features at higher frequencies $f \approx 10^2$ THz, which are due to bond vibrations, which are not accounted for in the rigid-bond classical water models we consider.

## S7. VISCOSITY SPECTRUM OF A RIGID-BODY LENNARD-JONES FLUID

To show how the polarity of individual water molecules influences the viscosity spectrum, we compare the full water spectrum to that of an equivalent LJ fluid, obtained by setting the charges of the standard TIP4P/2005 water model to zero, and otherwise leaving all simulation parameters fixed. Since only the oxygen atoms of TIP4P/2005 water interact via a LJ potential, the resulting system is a LJ fluid. As the high density of water at standard pressure and temperature is only possible due to the electrostatic interaction, one obtains a very high pressure of $P \approx 12.500$ bar if the box volume remains unchanged. Therefore, we also simulate a system with a significantly lower temperature of $T = 80$ K, which results in a pressure of $P \approx -13$ bar, close to standard conditions of 1 atm used in the water simulations.

In the resulting viscosity spectra, shown in Fig. S5, one can clearly see that the second peak vanishes, as expected if our interpretation of the water spectrum (where this peak is associated with hydrogen-bond vibrations and librational oscillations) holds. This indicates that the polarity of water molecules leads to a coupling between translation and rotation of individual molecules within the hydrogen-bond network, which induces a coupling between oscillations within the hydrogen-bond network and the shear viscosity.

The main Maxwell peak, which for water is at $f \approx 0.2$ THz, shifts towards higher frequencies for the LJ fluid; according to our interpretation of this peak as being associated with nearest-neighbor escape barrier hopping, this means that for the LJ fluid a particle escapes, on average, more quickly from its current position as compared to a water molecule. This is consistent with the fact that the hydrogen-bond network of water locally stabilizes the position of individual fluid molecules.

[1] S. Pronk, S. Páll, R. Schulz, P. Larsson, P. Bjelkmar, R. Apostolov, M. R. Shirts, J. C. Smith, P. M. Kasson, D. v. d. Spoel, B. Hess, and E. Lindahl, Bioinformatics **29**, 845 (2013).
[2] T. Darden, D. York, and L. Pedersen, The Journal of Chemical Physics **98**, 10089 (1993).
[3] G. Bussi, D. Donadio, and M. Parrinello, The Journal of Chemical Physics **126**, 014101 (2007).
[4] M. Parrinello and A. Rahman, Journal of Applied Physics **52**, 7182 (1981).
[5] A. K. Malde, L. Zuo, M. Breeze, M. Stroet, D. Poger, P. C. Nair, C. Oostenbrink, and A. E. Mark, Journal of Chemical Theory and Computation **7**, 4026 (2011).
[6] C. Oostenbrink, A. Villa, A. E. Mark, and W. F. Van Gunsteren, Journal of Computational Chemistry **25**, 1656 (2004).
[7] J. L. F. Abascal and C. Vega, The Journal of Chemical Physics **123**, 234505 (2005).
[8] R. Zwanzig, Annual Review of Physical Chemistry **16**, 67 (1965).
[9] D. J. Evans and G. Morriss, *Statistical Mechanics of Nonequilibrium Liquids* (2008).
[10] J.-P. Hansen and I. R. McDonald, *Theory of Simple Liquids* (Elsevier, 1990).

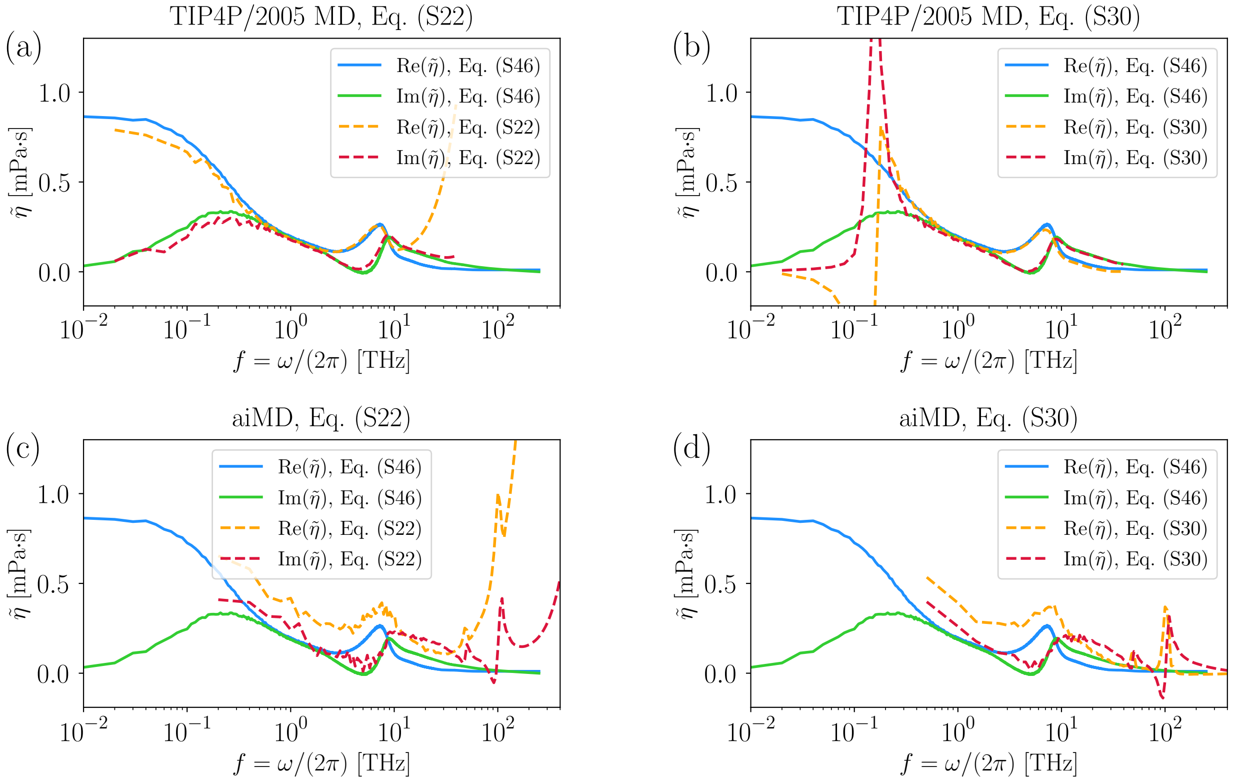


FIG. S4. **Viscosity spectra at finite wave number $k$.** In all subplots, the blue and green solid lines denote the real- and imaginary parts of the viscosity spectrum of TIP4P/2005 water at $k = 0$, calculated using Eq. (S46) and shown in Fig. 4 (a) of the main text. **(a), (b)** From force field MD simulations of 128 water molecules in a cubic box of edge length $L = 1.56$ nm, and with an interaction cut-off distance of 0.75 nm, the space-averaged transversal current is calculated via Eqs. (S55), (S56); using the corresponding normalized autocorrelation function, the viscosity spectrum at $k = 4.016\,\mathrm{nm}^{-1}$ is calculated using **(a)** Eq. (S22), and **(b)** Eq. (S30). **(c), (d)** From aiMD simulations of 128 water molecules in a box of edge length $L = 1.56$ nm, the space-averaged transversal current is calculated via Eqs. (S55), (S56); using the corresponding normalized autocorrelation function, the viscosity spectrum at $k = 4.016\,\mathrm{nm}^{-1}$ is calculated using **(c)** Eq. (S22), and **(d)** Eq. (S30).

[11] R. M. Christensen, *Theory of Viscoelasticity* (Courier Corporation, 2003).
[12] R. Zwanzig, *Nonequilibrium Statistical Mechanics* (Oxford University Press, USA, 2001).
[13] This can be understood by thinking of $\hat{f}(0)\hat{g}(0)$ as the Fourier transform (here denoted by $\mathcal{F}$) of the convolution (here denoted by $*$), evaluated at zero: $\hat{f}(\mathbf{0})\hat{g}(\mathbf{0}) = \mathcal{F}(f * g)(\mathbf{0}) = \left[\int \mathrm{d}^3\mathbf{x}\ \exp\left[i\mathbf{k}\cdot\mathbf{x}\right](f * g)(\mathbf{x})\right]|_{\mathbf{k}=\mathbf{0}} = \int \mathrm{d}^3\mathbf{x} \int \mathrm{d}^3\mathbf{y}\ f(\mathbf{y})g(\mathbf{x}-\mathbf{y}) = \int \mathrm{d}^3\mathbf{x} \int \mathrm{d}^3\mathbf{y} f(\mathbf{y})g(\mathbf{x}-\mathbf{y}) = V^2\left[1/V^2 \int \mathrm{d}^3\mathbf{x} \int \mathrm{d}^3\mathbf{x}'\ f(\mathbf{x})g(\mathbf{x}')\right]$.
[14] P. J. Daivis and D. J. Evans, The Journal of Chemical Physics **100**, 541 (1994).
[15] M. Mondello and G. S. Grest, The Journal of Chemical Physics **106**, 9327 (1997).
[16] T. Chen, B. Smit, and A. T. Bell, The Journal of Chemical Physics **131**, 246101 (2009).
[17] H. J. C. Berendsen, J. R. Grigera, and T. P. Straatsma, The Journal of Physical Chemistry **91**, 6269 (1987).
[18] M. Heyden, J. Sun, S. Funkner, G. Mathias, H. Forbert, M. Havenith, and D. Marx, Proceedings of the National Academy of Sciences **107**, 12068 (2010).
[19] J. O. Daldrop, M. Saita, M. Heyden, V. A. Lorenz-Fonfria, J. Heberle, and R. R. Netz, Nature Communications **9** (2018), 10.1038/s41467-017-02669-9.
[20] B. J. Palmer, Physical Review E **49**, 359 (1994).

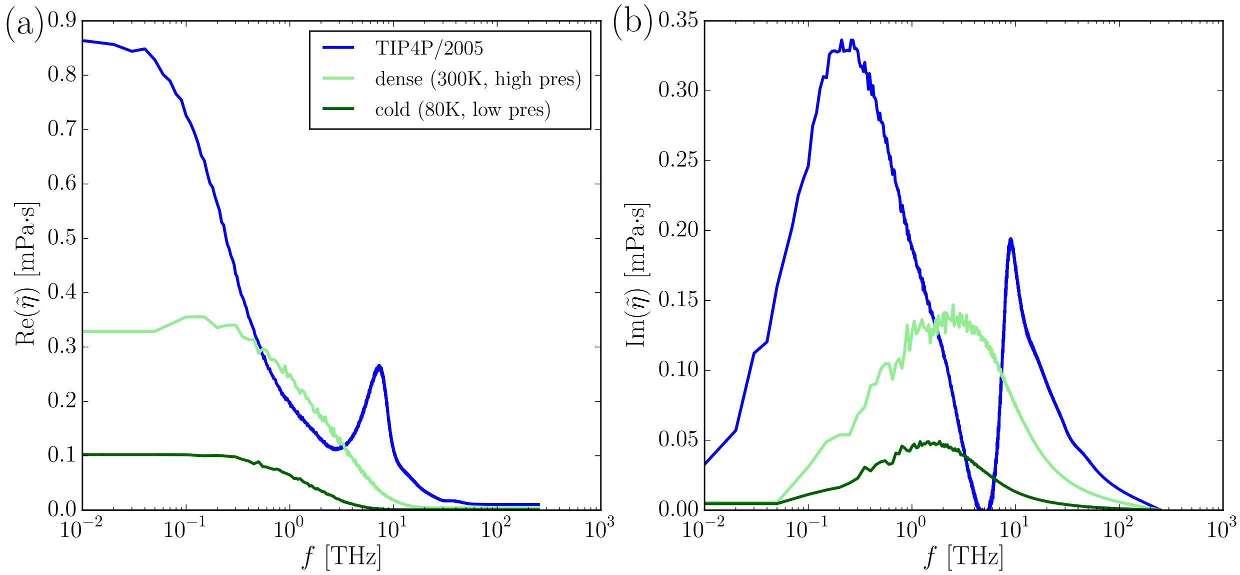


FIG. S5. Viscosity spectrum of TIP4P/2005 water (replot of Fig. 4 (a) of the main text), together with viscosity spectra of a LJ fluid at two different temperatures. Subplot (a) shows the real part of the spectrum, subplot (b) shows the imaginary part. Spectra are calculated using Eq. (S46). For discussion, see Sect. S7.
